# Supplementary material for: Subdimensional Expansion for Multi-objective Multi-agent Path Finding
Source: arXiv:2102.01353 source file (2021-07-10)
Supplement: Supplementary file 1 [file appendix.tex]

To prove Theorem \ref{thm:find_all_pareto}, we introduce a few lemmas at first.

\begin{lemma}\label{lem:terminate}
	If there is no conflict-free path connecting $v_o$ and $v_f$, MOM* terminates in finite time without returning a path.
\end{lemma}

\begin{proof}
	During the search, any states involved in agent-agent conflicts are never inserted into OPEN (line 15-16 in Algorirthm \ref{alg:mom*}) and thus MOM* never return a path with conflicts. 
	
	MOM* conducts A*-like search and visits every joint vertex in $G^{sch}$ unless $G^{sch}$ is modified when collision set of a state grows. For a state $s$, its collision set $I_C(s)$ can grow at most $(N-1)$ times until $I_C(s)=I$. In addition, since $G^i, i\in I$ are finite (and thus $G$ and $G^{sch}$ are finite), there is a finite number (denoted as $K$) of Pareto-optimal joint paths in $G$ from $v_o$ to any joint vertex $v \in V$.
%	For each agent, the length of its individual path from $v^i_o$ to any vertex $v^i \in V^i$ is at most $V_{max}=\max_{i\in I}|V^i|$. Let $d_{max}$ denote the maximum degree (in-degree for directed graphs) of any vertices in any individual graph. So there are at most $d_{max}^{V_{max}}$ individual Pareto optimal paths from $v^i_o$ to any vertex $v^i_k \in V^i$ and there are at most $d_{max}^{V_{max}N}$ joint Pareto optimal paths from $v_o$ to any joint vertex $v_k \in V$.
	There are totally $|V|$ joint vertices in $G$. Thus, $G^{sch}$ can be modified for at most $(N-1)|V|K$ times, which is a finite number. If there is no solution in $G$, then MOM* terminates in finite time. \footnote{Some readers may wonder why there is no need to bound the time horizon for search. To explain that, we just need to show that an agents can not wait-in-place for an arbitrary amount of time. Notice that the cost vector associated with wait-in-place, which is a self-loop, is strictly positive. Thus the cost vector of a joint path $\pi_1$ with unnecessary waits must be dominated by a corresponding joint path $\pi_2$ without those unnecessary waits and $\pi_1$ is guaranteed to be pruned. So there is no need to bound the maximum time horizon for search.}
\end{proof}

Let $succ(v^i_k)|_{\pi}$ and $succ(v_k)|_{\pi}$ denote the successor individual vertex of $v^i_k$ and successor joint vertex of $v_k$ along joint path $\pi$ respectively. 
Similarly, let $prec(v^i_k)|_{\pi}$ and $prec(v_k)|_{\pi}$ denote the predecessor individual vertex of $v^i_k$ and predecessor joint vertex of $v_k$ along $\pi$ respectively. When the context is clear, we omit $|_{\pi}$ and use $succ(\cdot)$ and $pred(\cdot)$ to indicate some successor and predecessor of a vertex.

\begin{lemma}\label{lem:stop_expand}
	For any state $s_l=(v_l,g_l)$ that is generated during the limited neighbor expansion (line 10 in Algorithm \ref{alg:mom*}), if $s_l$ is not expanded, one of the following four cases must hold:\\ % generated means either generated from expansion or re-open in collision back propagation.
	(1) (pruned by filtering) there is a state $s_l'=(v_l',g_l')$ that reaches goal ($v_l'=v_f$) and $g_l' \succeq g_l + h(v_l)$.\\
	(2) (pruned by dominance) there is a state $s_l'=(v_l',g_l')$ that has the same joint vertex as $s_l$, $i.e.$ $v_l'=v_l$ and $g_l' \succeq g_l$.\\
	(3) (pruned by collision) there is a conflict between $pred(v_l)$ and $v_l$, $i.e.$ $\Psi(pred(v_l),v_l) \neq \emptyset$.\\
	(4) (find a solution) $v_l=v_f$ and a solution is found.
\end{lemma}

\begin{proof}
This corollary comes from the construction of the Algorithm \ref{alg:mom*}. For any states $s_l \neq s_o$, it is generated at line 10 in Algorithm \ref{alg:mom*}. If there is conflict, $i.e.$ $\Psi(pred(v_l),v_l) \neq \emptyset$, $s_l$ is discarded and thus not expanded (line 16), which is case (3). If state $s_l$ is not in conflict, $s_k$ is insert into OPEN unless get pruned by dominance (line 17), which is case (2). For any states that enters OPEN, it either be pruned in procedure {FilterOpen} (line 8), which is case (1) or get popped eventually. For any state that is popped from OPEN, it either reaches goal $v_l=v_f$ and represents a non-dominated solution (line 6), or get expanded.
\end{proof}

\textbf{Remarks} Notice that Lemma \ref{lem:stop_expand} rules out the initial state $s_o$ which is generated from initialization (not from limited neighbor expansion). This only matters at the edge case where goal and start overlaps, $i.e.$ $v_o=v_f$, which makes MOM* terminates immediately as initial state $s_o$ reaches $v_f$ and return a trivial solution with length one. MOM* works correctly for this edge case. Therefore, we rule out this trivial edge case for the rest of the analysis. %Secondly, a state can be closed and re-open many times due to collision set back-propagation

\begin{lemma}\label{lem:all_found}
	All Pareto-optimal joint paths contained in $G^{sch}$ are found by MOM*.
\end{lemma}

\begin{proof}
	MOM* conducts {\it complete} search within $G^{sch}$ given a joint vertex by examining all limited neighbors. 
	From Lemma \ref{lem:terminate}, MOM* terminates in finite time, thus all generated search states end up with one of the cases in Lemma \ref{lem:stop_expand}. We prove by showing that none of the first three cases in Lemma \ref{lem:stop_expand} leads to a $\pi_* \in \Pi_*$ and therefore MOM* never prune a state that leads to a $\pi_* \in \Pi_*$. All other states that fall in case (4) represent a $\pi_* \in \Pi_*$.
	
	For case (1), if candidate state $s_k$ is filtered by $s_l=(v_l,g_l)$ that reaches goal ($v_l=v_f$) and $g_l \succeq g_k + h(v_k)$, let $\pi'$ be an arbitrary path that connects $v_o$ and $v_f$ via $s_k$, thus $g_l \succeq g_k + h(v_k) \succeq g_k + g(\pi'(v_k,v_f)) = g(\pi') $ and thus $\pi' \notin \Pi_*$.
	
	For case (2), if candidate state $s_k$ is dominated by state $s_l=(v_l,g_l)$ that has the same joint vertex as $s_k$, $i.e.$ $v_l=v_k$ and $g_l \succeq g_k$, let $\pi'$ be an arbitrary path that connects $s_o$ and $s_f$ via $s_k$, thus $g_l + g(\pi'(s_k,s_f)) \succeq g_k + g(\pi'(s_k,s_f)) = g(\pi') $ and thus $\pi' \notin \Pi_*$.
	
	For case (3), as candidate state $s_k$ leads to conflicts, $s_k$ cannot be part of conflict-free path and thus not part of $\Pi_*$.
\end{proof}

\begin{lemma}\label{lem:not_contained}
	If a Pareto path $\pi_*$ is not contained in $G^{sch}$, there exists a state $s_k=(v_k,g_k)$ along $\pi_*$ such that, for at least one agent $j \in I$, (1) $j \notin I_C(s_k)$ and (2) $succ(v^j_k)|_{\pi_*} \notin \phi^j(v^j_k)$.
\end{lemma}

\begin{proof}
	We prove this by contradiction. If $j \in I_C(s_k)$, by the definition of limited neighbors, all possible neighbors in $G^j$ is included into $G^{sch}$ and $succ(v_k)|\pi_*$ is included into $G^{sch}$. If $succ(v^j_k)|_{\pi_*} \in \phi^i(v^j_k)$, then by the definition of limited neighbors, edge connecting $v^j_k$ and $succ(v^j_k)|_{\pi_*}$ is contained in $G^{sch}$. Therefore, assuming either of the case holds for all states along $\pi_*$, then $\pi_*$ is included into $G^{sch}$, which leads to constradiction.
\end{proof}

If a $\pi_*$ is not contained in $G^{sch}$, define ``non-complete state'' to be the state $s_k=(v_k,g_k)$ as described in Lemma \ref{lem:not_contained}.
%along $\pi_*$ such that, for at least one agent $j \in I$, (1) $i$ is not contained in the collision set, $i.e.$ $j \notin I_C(s_k)$ and (2) the successor individual vertex of $v^j_k$ along $\pi_*$ is not contained in Pareto policy, $i.e.$ $succ(v^j_k)|_{\pi_*} \notin \phi^j(v^j_k)$. 
Define ``non-complete agents'', symbolically $I_j(s_k)$, to be the set of all agents as described in Lemma \ref{lem:not_contained}. With those definitions in hand, Lemma \ref{lem:not_contained} can be formulated as: If a Pareto path $\pi_*$ is not contained in $G^{sch}$, there exists a non-complete state $s_k$ and a corresponding non-empty set of non-complete agents $I_j(s_k) \neq \emptyset$.

Let $\pi_\phi^i(v_k,v_l)$ denote an individual Pareto optimal path connecting $v_k$ and $v_l$ ignoring any other agents and let $I_{\Omega}$ be an arbitrary subset of index set, $i.e.$ $I_{\Omega} \subseteq I$. Given a conflict-free path $\pi(v_k,v_l)$, let $\pi^{I_\Omega}(v_k,v_l)$ be a path (which might contains conflicts) constructed as follows: \\
(1) for all $i \notin I_{\Omega}$, agent $i$ follows an arbitrary individual Pareto path, noted as  $\pi_\phi^i(v_k,v_l)$, ignoring any agent-agent conflicts.\\
(2) for all $i \in I_{\Omega}$, agent $i$ follows its individual path $\pi^i(v_k,v_l)$ as contained in $\pi(v_k,v_l)$.

\begin{corollary}\label{coro:collision}
	For a feasible solution $\pi(v_{o},v_{f})$ and a subset of agents $I_{\Omega} \subseteq I$, if there exists along $\pi^{I_\Omega}(v_{o},v_{f})$ a state $s_k=(v_k,g_k)$ with non-empty collision set $ \Psi(v_k, succ(v_k)|_{\pi(v_{o},v_{f})}) \neq \emptyset$, then there exists $i \in \Psi(v_k, succ(v_k)|_{\pi(v_{o},v_{f})})$ such that $i \in I\backslash I_{\Omega}$. 
\end{corollary}

This corollary follows from the definition of $\pi^{I_\Omega}(v_{o},v_{f})$. All agents within set $I_\Omega$ follow the same individual paths as contained in $\pi(v_{o},v_{f})$, which is a feasible joint path, and thus cannot get involved into any conflicts. Any conflicts must be involved with an agent not in $I_{\Omega}$.

\begin{lemma}\label{lem:subset_compare}
	For any $\pi_* \in \Pi_*$, if $\pi_*$ is not contained in $G^{sch}$, let $s_k$ and $I_j$ denote the non-complete state and the corresponding set of non-complete agents, let $I_\Omega = I \backslash I_j$, then $g(\pi_*^{I_\Omega}) \succeq g(\pi_*) $.
%	Given $I_{\Omega} \subseteq I$, for any $\pi_* \in \Pi_*$, 
%	%$ \pi_* \nsucceq \pi_*^{I_{\Omega}}$.
%	$ \pi_*^{I_{\Omega}} \succeq \pi_* $.
\end{lemma}

\begin{proof}
	By definition of $\pi_\phi^i(v_o,v_f)$, $g(\pi_\phi^i(v_o,v_f)) \succeq g(\pi_*^i), \forall i \in I_j$. 
	Thus $ g(\pi_*^{I_\Omega}) = \Sigma_{i \in I_{\Omega}}g(\pi_*^i) + \Sigma_{i \in I_j} g(\pi_\phi^i(v_o,v_f))  \succeq  \Sigma_{i \in I}g(\pi_*^i) = g(\pi_*)$. 
\end{proof}

%Let $B(s_l)$ represent the set of states that can be reached from $s_l$ by iteratively following the back\_set when a collision set is back-propagated. If $s_k \in B(s_l)$, it means that any conflicts detected in $\Psi(s_l,succ(s_l))$ can be back propagated to $s_k$ and therefore update $I_C(s_k)$. As an edge case, define $s_l \in B(s_l)$ which means conflict detected at $\Psi(s_l,succ(s_l))$ can update $I_C(s_l)$.

Let $\xi(s_l, s_k)$ be a ``back-propagation path'' from $s_l$ to $s_k$ which can be constructed by iteratively following back set of states. If $\xi(s_l, s_k)$ exists, it means that any conflicts detected at $\Psi(s_l,succ(s_l))$ can be back propagated to $s_k$ and therefore update $I_C(s_k)$. As an edge case, let $\xi(s_k, s_k)$ be defined which means conflict detected at $\Psi(s_k,succ(s_k))$ can update $I_C(s_k)$.
Let $B(s_k)$ be a set of states where for any state $s_l \in B(s_k)$, there exists a back-propagation path $\xi(s_l, s_k)$ connects from $s_l$ to $s_k$.

\begin{lemma}\label{lem:finally_include}
	Before MOM* terminates, all $\pi_* \in \Pi_*$ are included into $G^{sch}$.
%	MOM* expands a state $s_m=(v_m,g_m)$ such that $j \in \Psi(s_m, succ(s_m))$ and $s_m \in B(s_k)$.
\end{lemma}

\begin{proof}
	If a $\pi_* \in \Pi_*$ is not contained in $G^{sch}$, following Lemma \ref{lem:not_contained}, let $s_k$ and $I_j(s_k)$ denote a non-complete state and the set of non-complete agents. 
	We proceed by showing that, for all $j\in I_j(s_k)$, MOM* expands a state $s_m=(v_m,g_m)$ such that $j \in \Psi(s_m, succ(s_m))$ and $s_m \in B(s_k)$. Therefore, $I_C(s_k)$ is updated by back-propagation which makes $j\in I_C(s_k)$ and grows $G^{sch}$. $G^{sch}$ stops growing untill there exists neither non-complete agents nor non-complete states and all $\pi_*$ are included into $G^{sch}$.
	
	Let $I_\Omega = I \backslash I_j$, from Lemma \ref{lem:subset_compare}, $g(\pi_*^{I_\Omega}) \succeq g(\pi_*) $ and thus all states along $\pi_*^{I_\Omega}$ are generated and expanded one after another unless either of the cases in Lemma \ref{lem:stop_expand} happens. Considering Lemma \ref{lem:stop_expand}, for any states $s_l$ after $s_k$ along $\pi_*^{I_\Omega}$, case (1) and (4) can not happen because otherwise $\pi_*$ cannot be Pareto-optimal. 
	
	For case (3), first of all, from Corollary \ref{coro:collision}, any collision among agents within $I_\Omega$ are already resolved along $\pi_*^{I_\Omega}$. 
	Therefore, if case (3) happens, $j \in \Psi(s_m,succ(s_m)) $. Since $s_m$ is generated by following path $\pi_*^{I_\Omega}$ from $s_k$, thus $s_m \in B(s_k)$ and $I_C(s_k)$ is updated to include $j$, which grows $G^{sch}$.
	
	For case (2), let $s_l'=(v_l',g_l')$ represent the state that dominates $s_l=(v_l,g_l)$, $i.e.$ $g_l' \succeq g_l$ and $v_l'=v_l$. If $j \in I_C(s_l')$, then with dominance-based back-propagation (Algorithm \ref{alg.dom_back_prop}), $I_C(s_k)$ will be updated to include $j$. If $j \notin I_C(s_l')$, then $s_k$ is added to back\_set($s_l'$) and thus any states generated from $s_l'$ belongs to $B(s_k)$. Then, let $\pi^{I_\Omega} (v_l',v_f)$ denote a Pareto path from $s_l'$ to $v_f$. Along $\pi^{I_\Omega} (v_l',v_f)$, there must be conflict, because otherwise, from Lemma \ref{lem:subset_compare}, $g_l'+ g(\pi^{I_\Omega} (v_l',v_f))\succeq g_l + g(\pi_*^{I_\Omega} (v_l', v_f)) = g(\pi^*)$, which means $\pi^*$ is not Pareto-optimal. If there is a conflict, from Corollary \ref{coro:collision}, $j \in I_j$ must be involved in the conflict detected. Thus $I_C(s_k)$ is updated to include $j$, which grows $G^{sch}$.
\end{proof}

Now, we prove Theorem \ref{thm:find_all_pareto}.

\begin{proof}
	From Lemma \ref{lem:terminate}, if there is no path connecting $v_o$ to $v_f$, MOM* terminates in finite time.
	If there exists path connecting $v_o$ to $v_f$, from Lemma \ref{lem:all_found} and Lemma \ref{lem:finally_include}, any $\pi_* \in \Pi_*$ contained in $G^{sch}$ is found by MOM* and all Pareto paths $\pi_* \in \Pi_*$ are included into $G^{sch}$ eventually before termination of MOM*. Therefore, MOM* finds all Pareto paths connecting $v_o$ to $v_f$.
\end{proof}
